# Supplementary material for: Data-Uncertainty Guided Multi-Phase Learning for Semi-Supervised Object Detection
Source: arXiv:2103.16368 source file (2021-03-29)
Supplement: Supplementary file 1 [file main.tex]

%\documentclass[review]{cvpr2}
\documentclass[final]{cvpr2}

\usepackage{times}
\usepackage{epsfig}
\usepackage{graphicx}
\usepackage{amsmath}
\usepackage{amssymb}
\usepackage{mathrsfs}
\usepackage{makecell}
\usepackage{booktabs}
\usepackage{multirow}
\usepackage{caption}
\usepackage{algorithmicx}  
\usepackage{algorithm}
\usepackage{algpseudocode}  
\usepackage{enumitem}
%\usepackage{titlesec}
\usepackage{subcaption}

%\captionsetup[table]{font={stretch=0.8}} 
%\captionsetup[figure]{font={stretch=0.8}} 

%\titlespacing*{\section} {0pt}{9pt}{0pt}

%\setlength{\textfloatsep}{12pt}
%\setlength{\baselineskip}{0pt}
\renewcommand{\multirowsetup}{\centering}

\usepackage[pagebackref=true,breaklinks=true,colorlinks,bookmarks=false]{hyperref}

\newcommand{\tabincell}[2]{\begin{tabular}{@{}#1@{}}#2\end{tabular}} 

\def\cvprPaperID{1987} % *** Enter the CVPR Paper ID here
\def\confYear{CVPR 2021}
%\setcounter{page}{4321} % For final version only


\begin{document}

%%%%%%%%% TITLE
\title{Supplementary Material for ``Data-Uncertainty Guided Multi-Phase Learning for Semi-Supervised Object Detection"}

\maketitle

\section{Visualization of Label Noise Overfitting Problem}

We select some images to further explain the label noise overfitting problem. The examples are in Fig. \ref{fig:of}. In the first case, the supervised model mislabels the aeroplane as a car, and we notice that the semi-supervised model trained with this pseudo label detects one more car that does not exist. In the second case, the supervised model thinks a part of the iron mesh is a person. This may be an accident mistake. However, in the results from the semi-supervised model, more parts of the iron mesh are detected as persons. The same thing also happens in other cases. The noisy pseudo labels generated by the FS model are regarded as the correct ones by the SSOD model. The SSOD then overfits to these noisy labels, a nature of deep learning neural networks. In the test stage, the SSOD model just tries to intimate the noisy labels used for training, thus generates more similar mistakes. These examples validate the label noise overfitting problem.

\begin{figure}[h]
   \centering
      \setlength{\abovecaptionskip}{5pt}
   \setlength{\belowcaptionskip}{0pt}
   \includegraphics[width=\columnwidth]{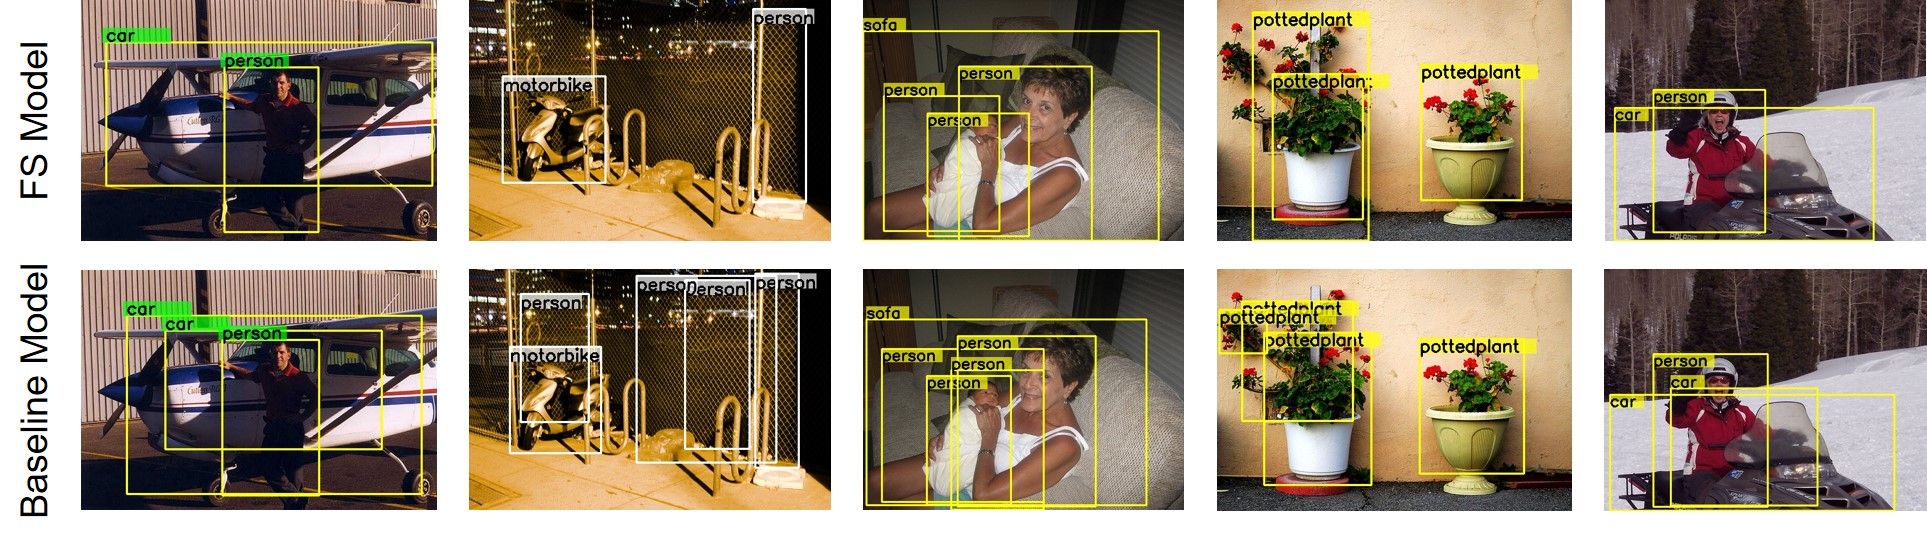}
   \caption{\textbf{Examples to explain the label noise overfitting problem.} The first row is pseudo labels from supervised model, and the second row is from semi-supervised model (baseline method). Because of the label noise overfitting problem, pseudo labels from the semi-supervised model contain more similar mistakes.}
   \label{fig:of}
\end{figure}

Because of the label noise overfitting problem, the detector is easy to concentrate on difficult images with more noise and uncertain regions where groundtruth labels are missed, while ignoring easy images and certain regions. Therefore, at \emph{image level}, we propose \textbf{a multi-phase learning method guided by uncertainty based image selection} to adopt multiple models handling easy and difficult images separately; at \emph{region level}, we present \textbf{a region uncertainty based RoI Re-weighting strategy} to further guide the SSOD training and force the model into more certain regions. 

\section{Quantitative Results}

\subsection{Extensive Comparison with Existing Methods}

To evaluate our method more comprehensively, we perform more experiments for SSOD on ResNet101 \cite{he2016deep} based Faster RCNN \cite{ren2015faster} and SSD512 \cite{liu2016ssd}, two more complicated models compared to ResNet50 based Faster RCNN and SSD300. The more extensive results are listed in Tab. \ref{tab:voc} and Tab. \ref{tab:coco}. 

For PASCAL VOC \cite{everingham2010pascal}, we observe that our method improves the mAP of the baseline method by 3\% on ResNet101 based Faster RCNN, from 76.6\% to 79.6\%, which is consistent with results on ResNet50. This demonstrates that our method can be applied to detectors with different backbones and validates the efficiency of our method. Compared to 78.6\% mAP with the ResNet50 backbone, ResNet101 achieves a higher mAP and has more potential for practical application. For SSD512, our method also manages to produce better predictions compared to state-of-the-art methods on one stage detectors and our method with SSD300. It is noticeable that the gap between our method (77.9\%) and the upper bound by fully-supervised learning on VOC0712 (79.6\%) is only 1.7\%, which further proves the strong ability of our method.



\begin{table}[]
\centering
\setlength{\abovecaptionskip}{2pt}
%\setlength{\belowcaptionskip}{0pt}
\caption{\textbf{Semi-supervised Detection Results on PASCAL VOC 2007 test} \emph{vs.} current SSOD methods and fully-supervised results trained on VOC07 or VOC0712. (L: labeled data, Un: unlabeled data.)}

\begin{minipage}[t]{\columnwidth}

%\begin{minipage}[t]{0.4\textwidth}
\resizebox{!}{0.13\columnwidth}{
\begin{tabular}{c|c|c|cc|c}
\Xhline{1pt}
Model & Backbone & Method & \tabincell{c}{L} & \tabincell{c}{Un} & mAP \\
\hline

\multirow{10}{1.2cm}{Faster RCNN}  & \multirow{5}{1.2cm}{ResNet50} & FS & VOC07 & - & 74.8  \\
 & & Baseline & VOC07 & VOC12 & 75.6\\
 & & DD \cite{radosavovic2018data} & VOC07 & VOC12 & 76.0\\
 & & ours & VOC07 & VOC12 & \textbf{78.6}\\
 & & FS & VOC0712 & - & 81.2\\
 
\cline{2-6}

 & \multirow{5}{1.2cm}{ResNet101} & FS & VOC07 & - & 76.1  \\
 & & Baseline & VOC07 & VOC12 &  76.6\\
 & & DD & VOC07 & VOC12 &  76.9\\
 & & ours & VOC07 & VOC12 & \textbf{79.6 }\\
 & & FS & VOC0712 & - &  82.2\\

\Xhline{1pt}
\end{tabular}
}
%\end{minipage}
\hfill
%\begin{minipage}[t]{0.4\textwidth}
\resizebox{!}{0.13\columnwidth}{
\begin{tabular}{c|c|c|cc|c}
\Xhline{1.2pt}
Model & Backbone & Method & \tabincell{c}{L} & \tabincell{c}{Un} & mAP \\
\hline

\multirow{6}{1.2cm}{SSD300}  & \multirow{12}{1.2cm}{VGG16 \cite{simonyan2014very}} & FS & VOC07 & - & 70.2\\ 
 & & Baseline & VOC07 & VOC12 & 71.8\\
 & & CSD \cite{jeong2019consistency} & VOC07 & VOC12 & 72.3\\
 & & ISD \cite{jeong2020interpolation} & VOC07 & VOC12 & 73.3\\
 & & ours & VOC07 & VOC12 & \textbf{74.5}\\ 
 & & FS & VOC0712 & - & 77.2\\

\cline{1-1}
\cline{3-6}

\multirow{6}{1.2cm}{SSD512}  & & FS & VOC07 & - & 73.3 \\ 
 & & Baseline & VOC07 & VOC12 &  74.8\\
 & & CSD  & VOC07 & VOC12 &  75.8\\
 & & ISD  & VOC07 & VOC12 &  76.4 \\
 & & ours & VOC07 & VOC12 & \textbf{77.9}\\ 
 & & FS & VOC0712 & - & 79.6 \\

\Xhline{1.2pt} 
\end{tabular}
}

\end{minipage}

\label{tab:voc}
\end{table}

For COCO \cite{lin2014microsoft}, we observe that our method persistently improves the mAP on objects with different scales of size, which demonstrates the strong generalization ability of our method. For different backbones or different data splits, our method consistently achieves better performance compared to existing SSOD methods. The most prominent phenomenon is that our method achieves 20.5\% on small objects with ResNet50 based Faster RCNN for co-35/80 split, while the corresponding fully-supervised upper bound is just 21.2\%. \textbf{The gap is only 0.7\%.} This demonstrates that our method learns knowledge within unlabeled images quite sufficiently, especially for some certain data. 



\begin{table}[]
\centering
\setlength{\abovecaptionskip}{2pt}
\caption{\textbf{Semi-supervised detection Results on COCO minival} \emph{vs.} current SSOD and FSOD results.}
\resizebox{0.85\columnwidth}{!}{
\begin{tabular}{c|c|cc|cccccc}
\Xhline{1.2pt}
Backbone & Method & \tabincell{c}{L} & \tabincell{c}{Un} & $AP$ & $AP_{50}$ & $AP_{75}$ & $AP_S$ & $AP_M$ & $AP_L$\\
\hline

\multirow{9}{1.3cm}{ResNet50} & FS & co-35 & - & 31.3 & 52.0 & 33.0 & 17.7 & 34.2 & 40.0\\
  & DD & co-35 & co-80 & 33.1 & 53.3 & 35.4 & 17.7 & 36.1 & 43.4\\
  & ours & co-35 & co-80 & \textbf{34.8} & \textbf{55.1} & \textbf{37.2} & \textbf{19.9} & \textbf{37.8} & \textbf{45.4}\\
  & ours + DD & co-35 & co-80 & \textbf{35.2} & \textbf{55.7} & \textbf{37.6} & \textbf{20.5} & \textbf{38.2} & \textbf{45.6}\\
  \cline{2-10}
  & FS & co-115 & - & 37.4 & 58.1 & 40.4 & 21.2 & 41.0 & 48.1\\
  & DD & co-115 & co-120 & 37.9 & 60.1 & 40.8 & 20.3 & 41.6 & 50.8\\
  & PL \cite{tang2020proposal} & co-115 & co-120 & 38.4 & 59.7 & 41.7 & 22.6 & 41.8 & 50.6\\
  & ours & co-115 & co-120 & \textbf{40.1} & \textbf{60.4} & \textbf{43.7} & \textbf{23.6} & \textbf{43.7} & \textbf{51.4}\\
  & ours + DD & co-115 & co-120 & \textbf{40.3} & \textbf{61.0} & \textbf{43.9} & \textbf{23.9} & \textbf{44.0} & \textbf{51.5}\\
\hline

\multirow{8}{1.3cm}{ResNet101} & FS & co-35 & - & 32.7 & 53.4 & 35.0 & 17.1 & 36.2 & 42.7\\
  & DD & co-35 & co-80 & 34.5  & 55.7  &  36.7 & 19.1 & 38.8 & 45.2\\
  & ours & co-35 & co-80 & \textbf{36.4} & \textbf{56.5} & \textbf{39.2} & \textbf{19.5} & \textbf{40.1} & \textbf{47.7}\\
  & ours + DD & co-35 & co-80 & \textbf{36.6} & \textbf{56.8} & \textbf{39.4} & \textbf{20.1} & \textbf{40.3} & \textbf{48.0}\\
\cline{2-10}

 & FS & co-115 & - & 39.4 & 60.1 & 43.1 & 22.4 & 43.7 & 51.1\\
  & DD & co-115 & co-120 & 40.1 & 62.1 & 43.5 & 21.7 & 44.3 & 53.7\\
  & ours & co-115 & co-120 & \textbf{42.2} & \textbf{62.5} & \textbf{46.1} & \textbf{25.0} & \textbf{46.7} & \textbf{54.5}\\
  & ours + DD & co-115 & co-120 & \textbf{42.3} & \textbf{62.7} & \textbf{46.3} & \textbf{25.3} & \textbf{46.7} & \textbf{54.9}\\
\Xhline{1.2pt} 
\end{tabular}
}
\label{tab:coco}
\end{table}



\subsection{Image Difficulty Distribution}


With recall/precision metric we propose in the original paper, the fraction of easy images is calculated and listed in Tab \ref{tab:easy}. For ResNet50 based Faster RCNN on PASCAL VOC, the fraction of easy images is 54\%, which is consistent with the result in our original paper where 50\% or 60\% easy images produce a higher mAP. If we combine our method with DD or use ResNet101 as the backbone, the quality of pseudo labels is higher, but we find that the easy data ratio is still close to 50\%. For more complicated datasets like COCO, the proportion of easy images is still approximately 50\%. This confirms that without any prior knowledge about the unlabeled dataset, 50\% is a good estimation of easy data.



\begin{table}[]
\centering
\setlength{\abovecaptionskip}{2pt}
\setlength{\belowcaptionskip}{0pt}
\caption{\textbf{Fraction of easy data proportion} on PASCAL VOC and MS COCO}
\resizebox{0.75\columnwidth}{!}{
\begin{tabular}{c|c|c|c|c}
\Xhline{1.2pt}
Dataset & Model & Backbone & DD & Easy Data Proportion \\
\hline

\multirow{4}{2.2cm}{PASCAL VOC}  & \multirow{4}{2.2cm}{Faster RCNN} & \multirow{2}{2.2cm}{ResNet50} &   & 54\% \\
  &  &  &\checkmark & 61\% \\
\cline{3-5}
  &  & \multirow{2}{2.2cm}{ResNet101} &   & 59\% \\
  &  &  &\checkmark & 64\% \\
%\cline{2-5}
%  & SSD300 & \multirow{2}{2.2cm}{VGG16} & & 53\% \\
%  & SSD512 &  & & 55\% \\ 
\hline 
\multirow{4}{2.2cm}{MS COCO}  & \multirow{4}{2.2cm}{Faster RCNN} & \multirow{2}{2.2cm}{ResNet50} &   & 46\% \\
  &  &  &\checkmark & 53\% \\
\cline{3-5}
  &  & \multirow{2}{2.2cm}{ResNet101} &   & 50\% \\
  &  &  &\checkmark & 56\% \\
\Xhline{1.2pt} 
\end{tabular}
}
\label{tab:easy}
\end{table}

\begin{figure}[]
   \centering
   \includegraphics[width=\columnwidth]{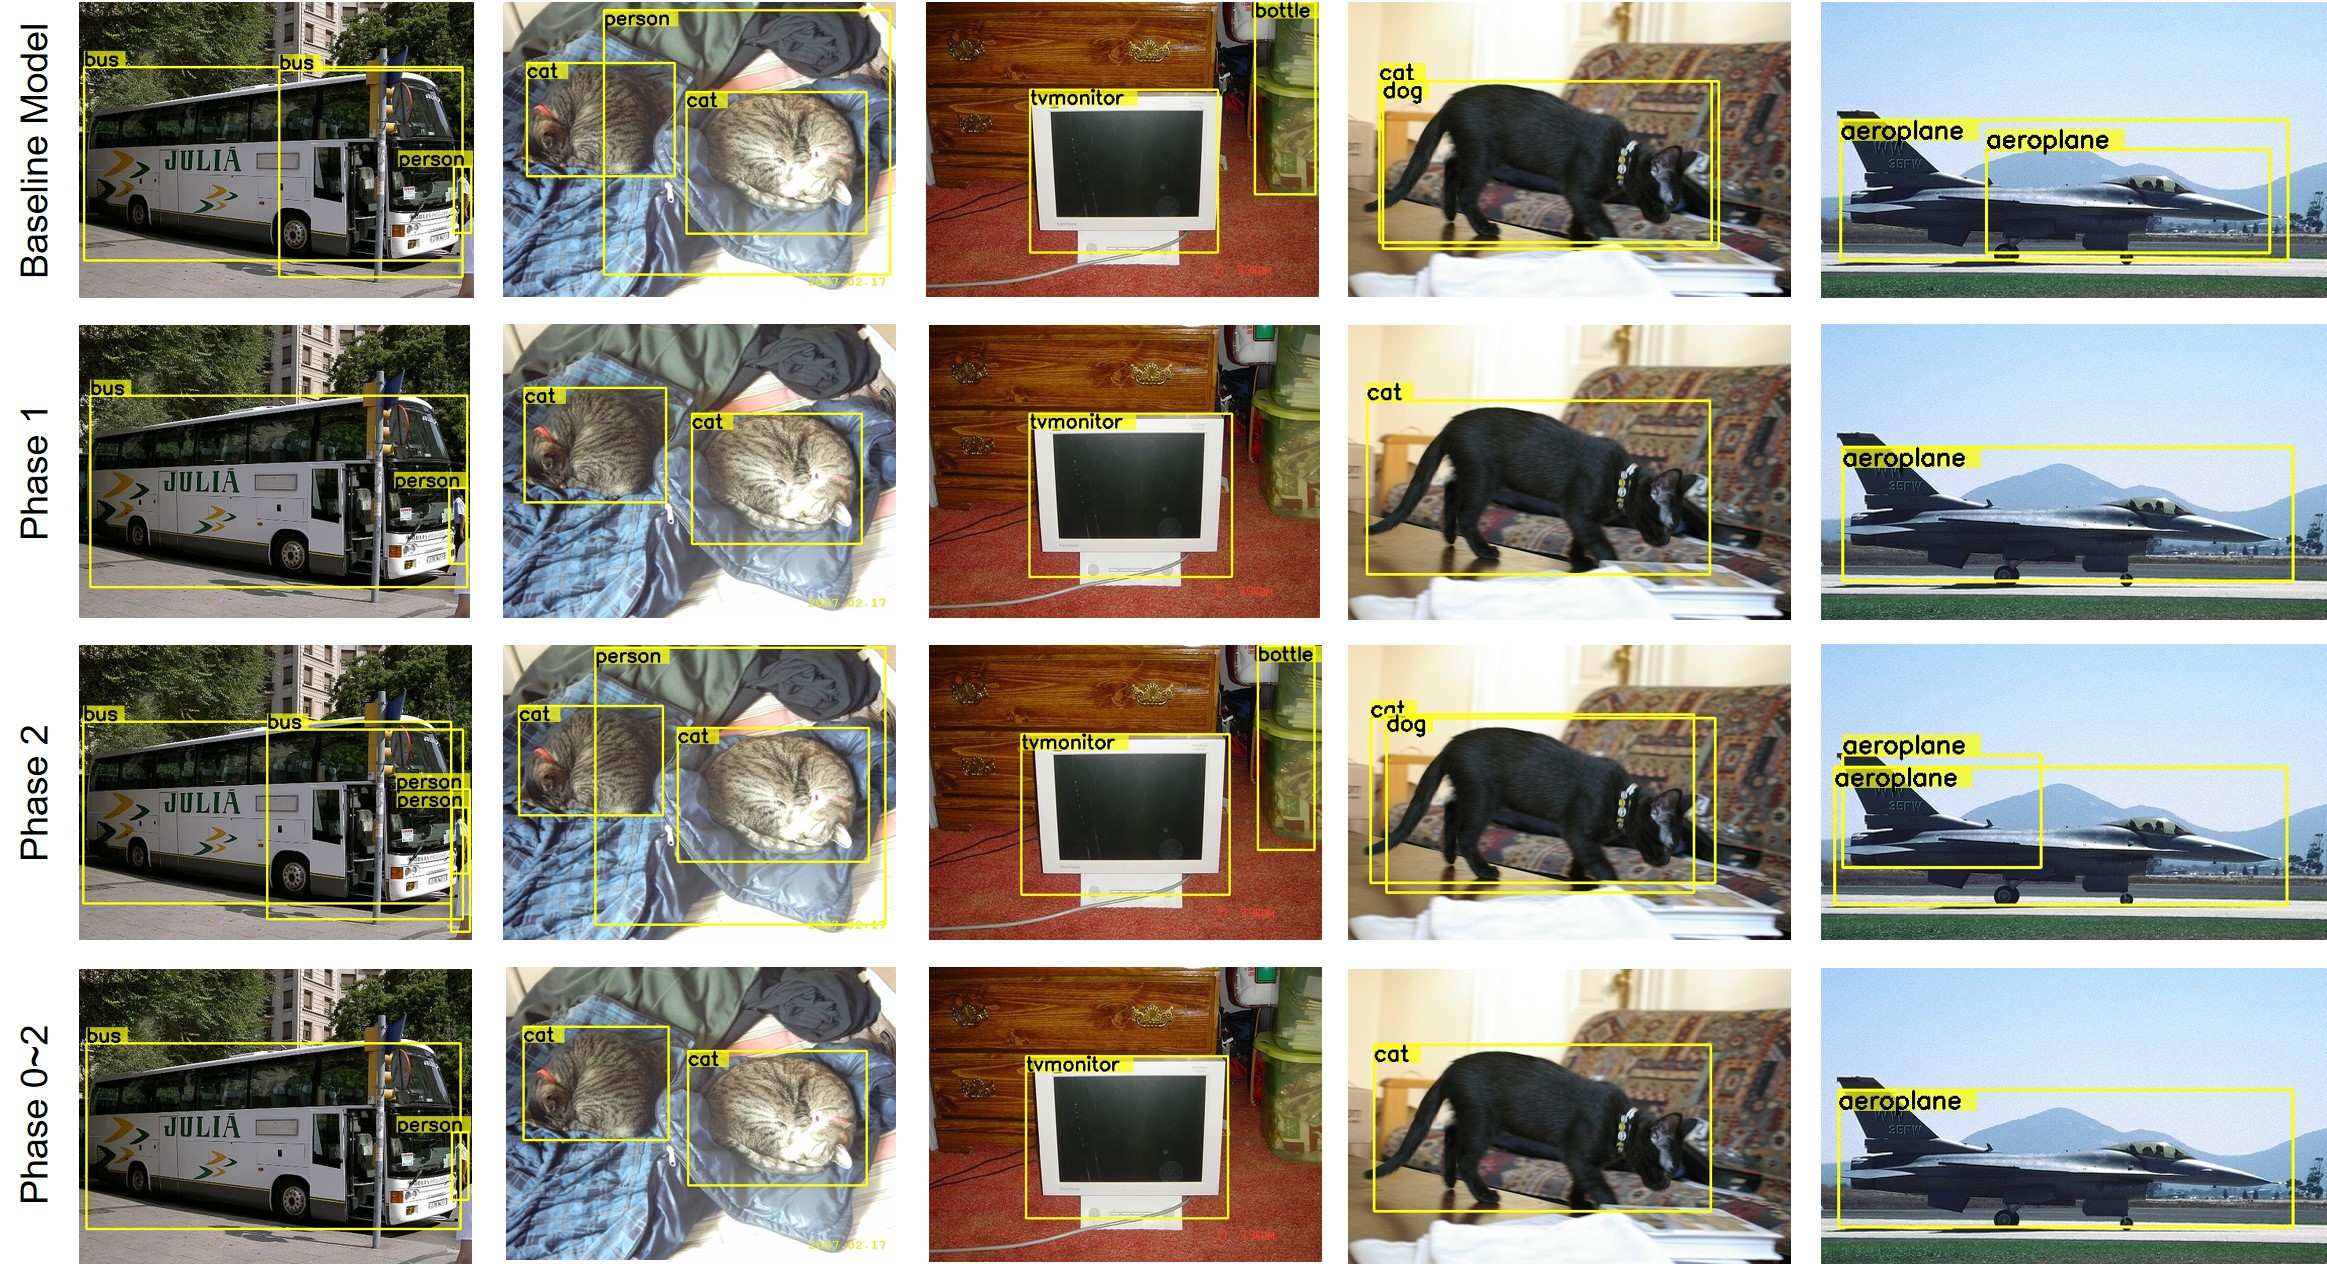}
   \caption{\textbf{Comparative examples on easy images.} The first row is from the baseline method, the second row is from the phase 1 model, the third row is from the phase 2 model, and the fourth row is from the phase ${0 \sim 2}$ model. The phase 1 model performs the best on these easy images, while the baseline model and the phase 2 model concentrates on difficult knowledge and makes mistakes on easy images.}
   \label{fig:easyimg}
\end{figure}

\begin{figure*}[]
   \centering
   \includegraphics[width=\columnwidth]{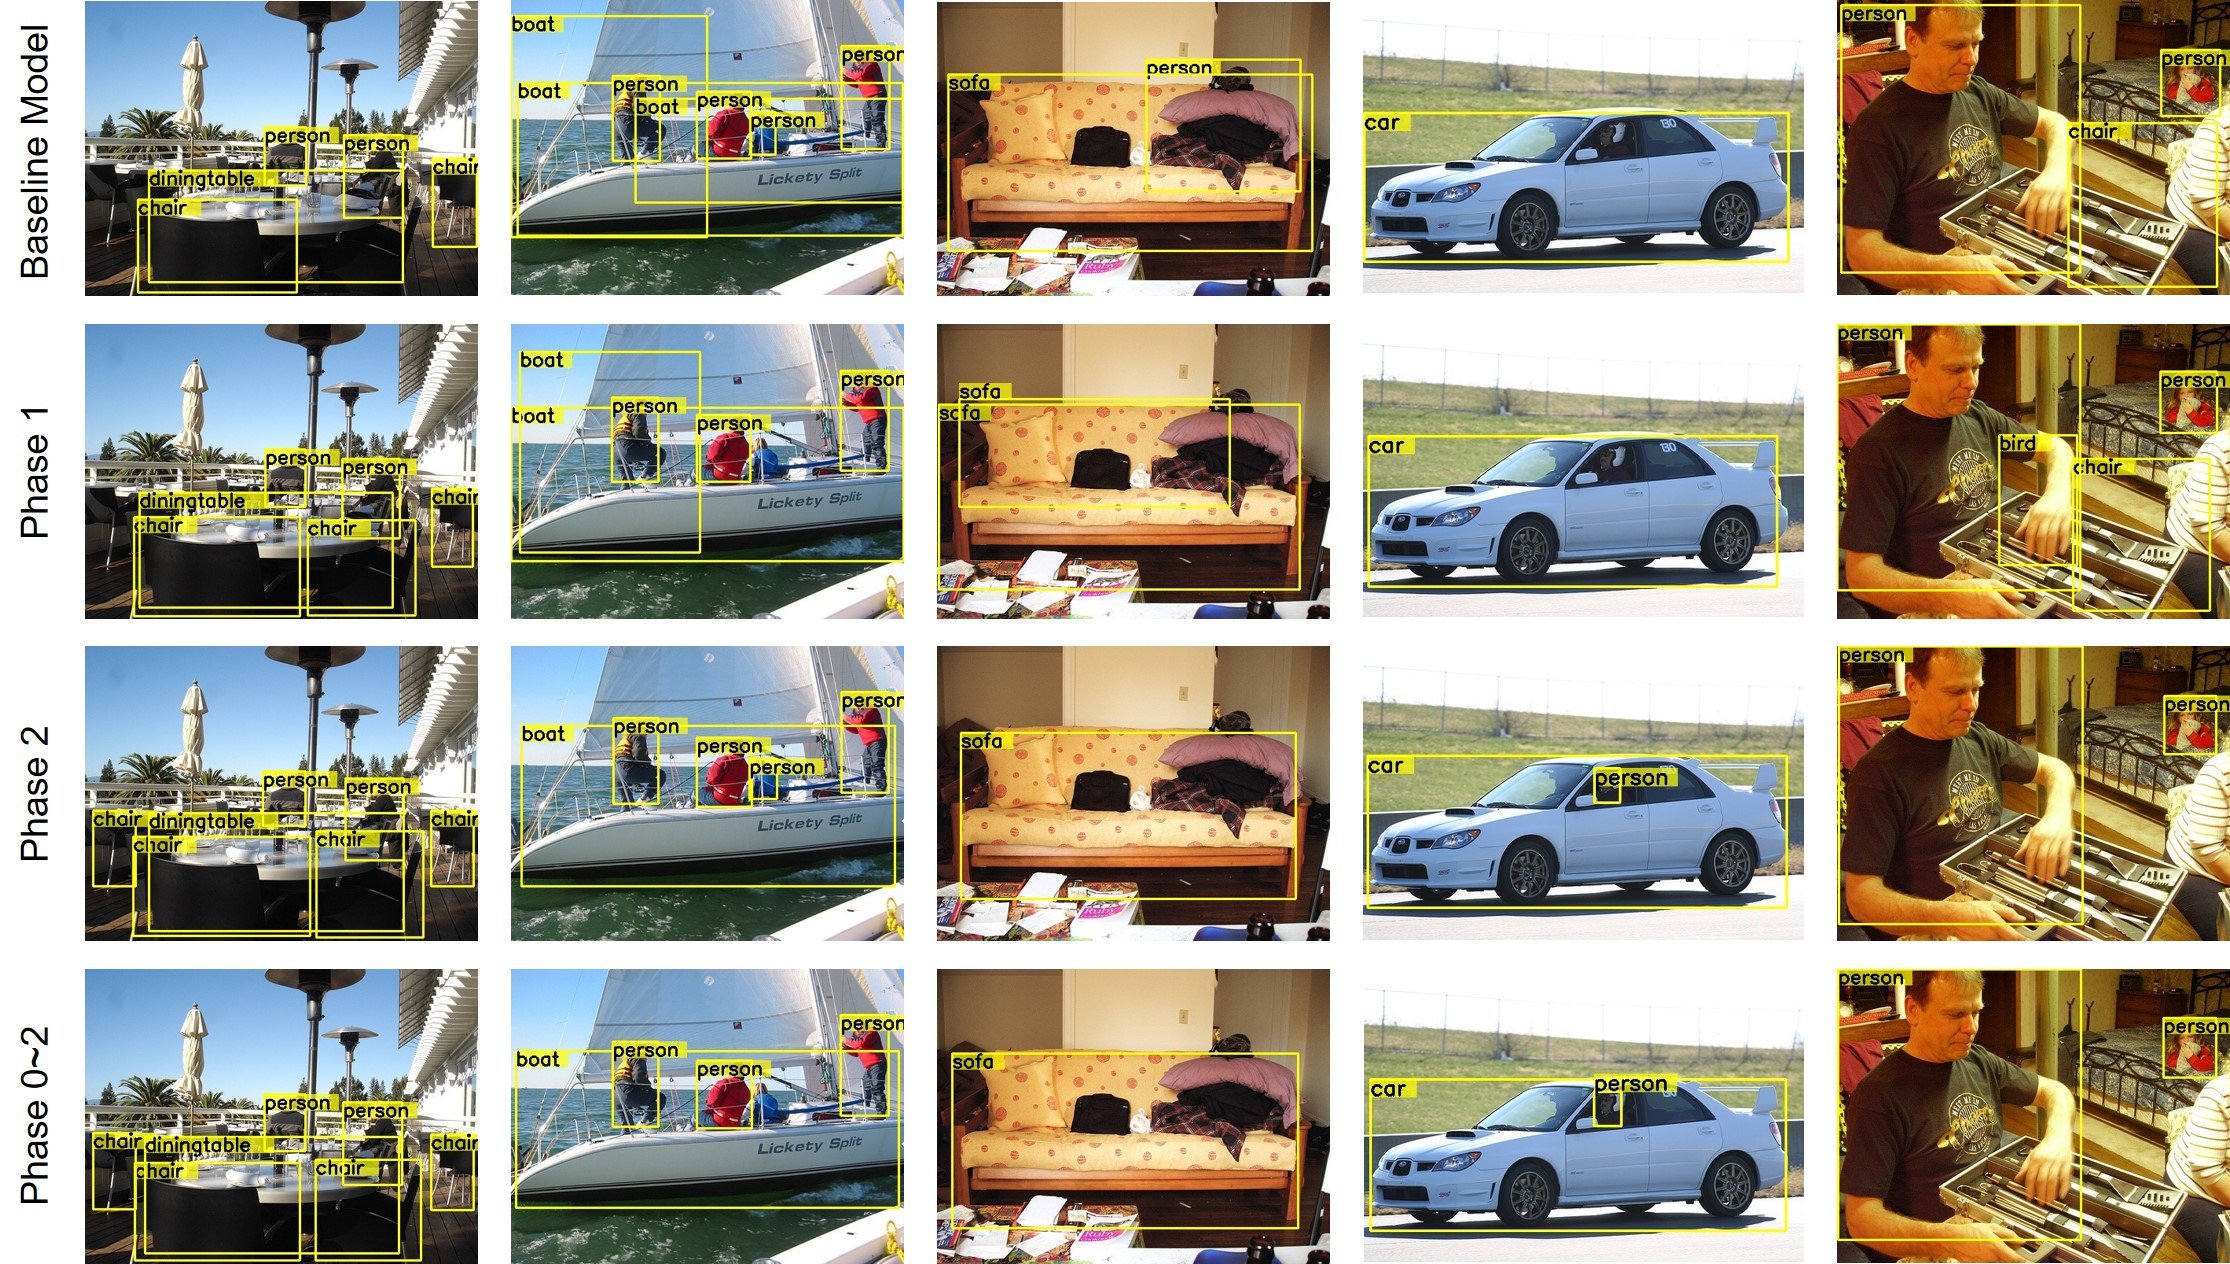}
   \caption{\textbf{Comparative examples on difficult images.} The first row is from the baseline method, the second row is from the phase 1 model, the third row is from the phase 2 model, and the fourth row is from the phase ${0 \sim 2}$ model. The phase 2 model performs the best on these difficult images, while the phase 1 model concentrates on easy knowledge and is not able to detect some confusing objects.}
   \label{fig:diffimg}
\end{figure*}



\section{Qualitative Results}

\subsection{Overall Visualized Results}

Fig. \ref{fig:easyimg} and Fig. \ref{fig:diffimg} shows the visualized results of baseline methods and our methods on several easy or difficult images. 

For easy images, we observe that the common points among them are that the objects within them are usually large and clear. The features for those objects are also obvious and they are not easy to be confused with other categories. We find that the detector from the first phase performs the best because they are trained with only easy unlabeled images and excel in easy knowledge. The baseline method and the second phase model both detect some extra objects that do not exist. This is because \textbf{these two models are trained with all unlabeled images and focus on difficult knowledge}. They thus keep a high vigilance and perform prediction even the corresponding region is only a little similar to those objects, such as the right 'bottle' in the third case. They are also easy to detect parts of the objects, such as the first and the fifth case. These images demonstrate that \textbf{the model from the first phase experts in easy knowledge.} After ensembling, the confidence scores of those redundant predictions are lowered down and they are not distinct in the final prediction. 

For difficult images, we find that the number of objects within them is a little large, or they contain some small and unclear objects. Some objects are easy to be confused with other categories or the background category. For example, the clothes in the third case look like a person, and the right small person in the fifth case is hard to distinguish from the environment. For these images, the second phase model is the best. The first phase model either makes some confusion or is not able to detect some objects. These images illustrate that \textbf{the model from the second phase learns difficult knowledge well.}

After ensembling, the model takes the advantage of all models thus is suitable for both easy and difficult images. Therefore, our method achieves a better result compared to the baseline method.


\begin{figure}[]
   \centering
   \includegraphics[width=\columnwidth]{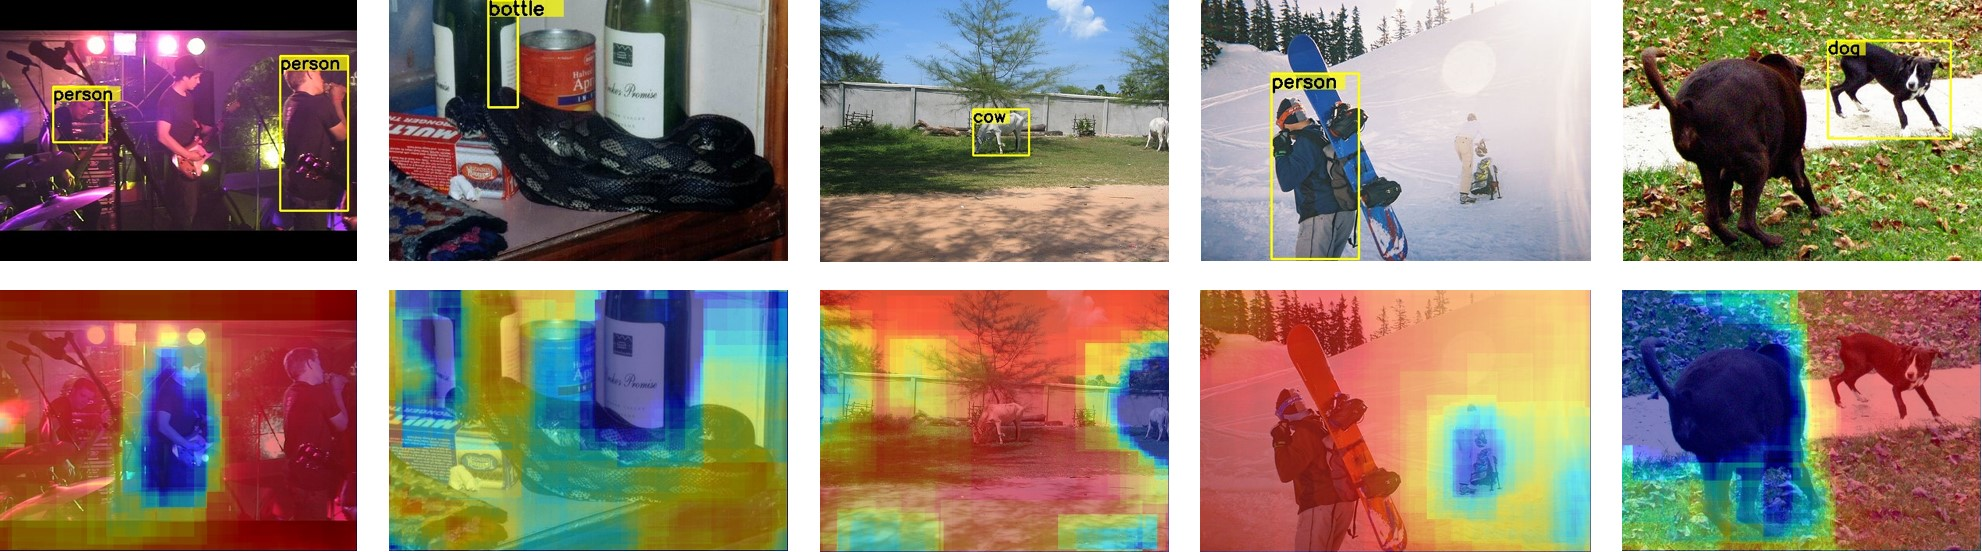}
   \caption{\textbf{Illustrative examples for RoI Re-weighting.} The first row is pseudo labels with missing annotation problem and the second row is heatmap for region uncertainty. Our method manages to detect uncertain regions (blue ones).}
   \label{fig:unreg}
\end{figure}


\subsection{Visualized Results for RoI Re-weighting}

We list more examples in Fig. \ref{fig:unreg}. We observe that our method also manages to detect uncertain regions where groundtruth labels are miss-annotated, such as the middle person for the first case, the bottles in the second case, the right cow in the third case, the right person in the fourth case, and the left dog in the fifth case. \textbf{Weights for these regions are reduced and incorrect gradient information deriving from uncertain regions is less likely to negatively affect the detector.}

From Fig. \ref{fig:rrimg}, we observe that with RoI Re-weighting, our model is able to detect more confusing and difficult objects compared to the model without RoI Re-weighting. This is just because that RoI Re-weighting helps the model avoid uncertain regions. Our model is less guided by uncertain and incorrect knowledge and is thus able to detect more difficult objects.

\begin{figure}[]
   \centering
   \includegraphics[width=\columnwidth]{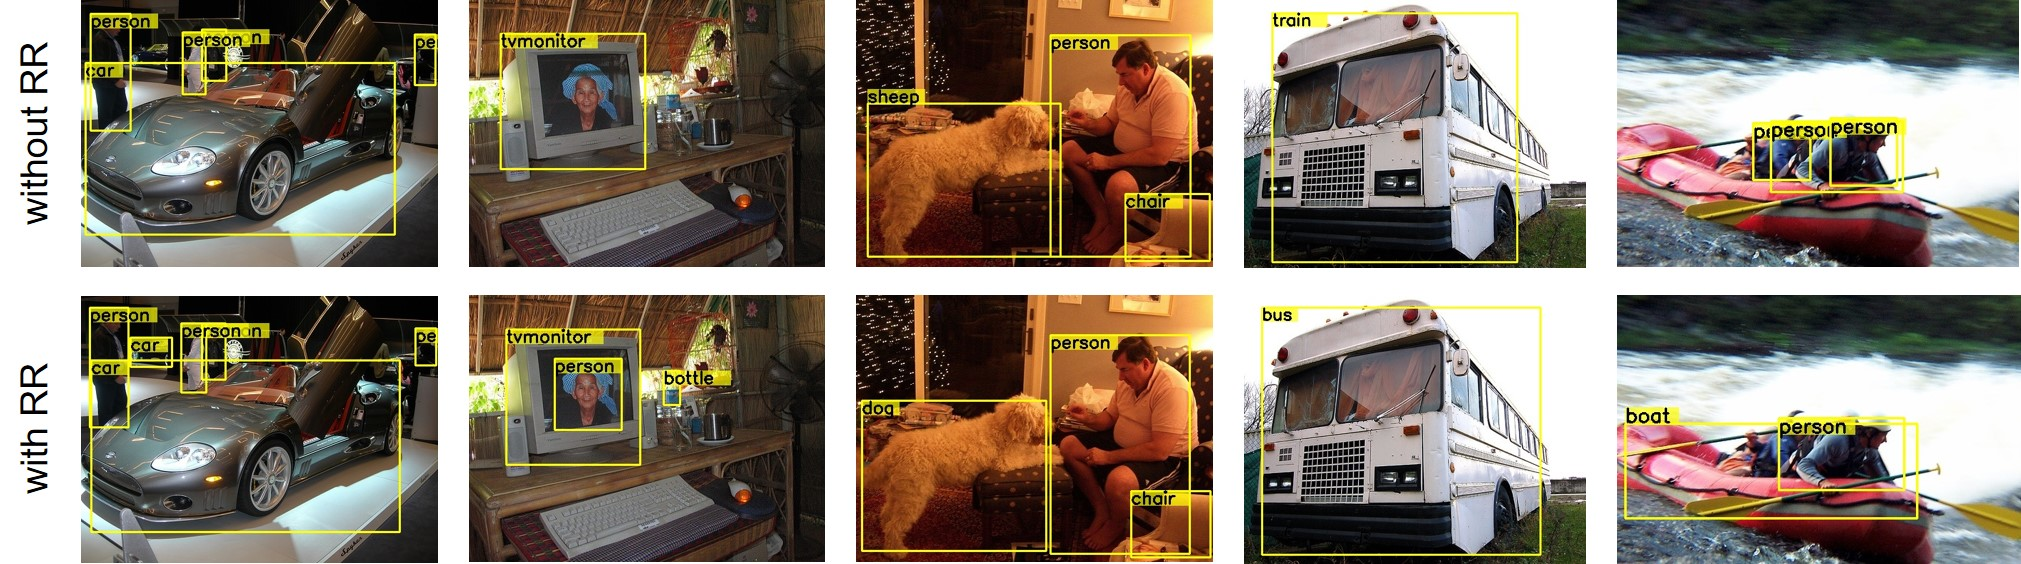}
   \caption{\textbf{Comparative examples for RoI Re-weighting.} The first row is from the two-phase model without RoI Re-weighting, and the second row is from the two-phase model with RoI Re-weighting. Because of RoI Re-weighting, the detector is able to handle more confusing objects.}
   \label{fig:rrimg}
\end{figure}



{\small
\bibliographystyle{ieee_fullname}
\bibliography{egbib}
}

\end{document}
